# Supplementary material for: Learning in Auctions: Regret is Hard, Envy is Easy
Source: arXiv:1511.01411 source file (2016-04-06)
Supplement: Supplementary file 1 [file appendix-low-dim.tex]

\begin{proofof}{Lemma \ref{lem:statistic-stability}}
We consider a specific sequence $\theta^{1:T}$ and a specific time-step $t$. For succinctness we we will denote with: 
\begin{align*}
\FTPL^t =~& \E_{x}\left[u( M(\{x\}\cup \theta^{1:{t-1}}), \theta^t)\right]\\
\BTPL^t =~& \E_{x}\left[u(M(\{x\}\cup \theta^{1:t}),\theta^t)\right]
\end{align*}
the expected reward of \emph{follow the perturbed leader} and \emph{be the perturbed leader}, correspondingly, at time-step $t$. We will also denote with $\phi^{t-1} =~ \phi(\theta^{1:t-1})$, $
\phi^t =~\phi(\theta^{1:t})$ and with $z=\phi(\{x\})$, the exponentially distributed random variable in $\R^d$. Thus we can re-write:
\begin{align*}
\FTPL^t =~& \E_{z}\left[u( M(z+\phi^{t-1}), \theta^t)\right]\\
\BTPL^t =~& \E_{x}\left[u(M(z+\phi^t),\theta^t)\right]
\end{align*}

We will construct a mapping $\mu:\R^d\rightarrow \R^d$, such that for any $z\in \R^d$:
\begin{equation}
M(z+\phi^{t}) = M(\mu(z)+\phi^{t-1})
\end{equation}
Observe that the two maximization problems are the same if we have that the vector ends up being the same, i.e., $\mu(z) = z + (\phi^{t}-\phi^{t-1})$. Observe that $\mu(x)$ is a bijection from $\R^d$ to $\R^d$. Thus we can write:
\begin{align*}
\FTPL^t=~& \int_{z\in \R^d}u(M(z+\phi^{t-1}),\theta^t) f(z) dz\\
=~&\int_{z\in \R^d}u(M(\mu(z)+\phi^{t-1}),\theta^t) f(\mu(z))  dz\\
=~&\int_{z\in \R^d}u(M(z+\phi^t),\theta^t) f(\mu(z))dz
\end{align*}
Now observe that for any $z\in \R^d$:
\begin{align*}
f(\mu(z)) =~& \exp\left\{-\epsilon\left(\|\mu(z)\|_1-\|z\|_1\right)\right\}f(z)\\
=~& \exp\left\{-\epsilon\left(\left\|z+\phi^t-\phi^{t-1}\right\|_1 -\|z\|_1\right)\right\} f(z)\\
\geq~&\exp\left\{-\epsilon\left\|\phi^t-\phi^{t-1}\right\|_1\right\} f(z)\\
\geq~&\exp\left\{-\epsilon D\right\} f(z)\\
\geq~&\left(1-\epsilon D\right) f(z)
\end{align*}
Plugging the above lower bounds in the integral we get:
\begin{align*}
\FTPL^t
\geq~& (1-\epsilon D)\int_{z\in \R^d}u(M(z+\phi^t),\theta^t) f(z)dz
= (1-\epsilon D)\cdot \BTPL^t \geq \BTPL^t - \epsilon D f_+(\theta^t)
\end{align*}
\end{proofof}
