# Supplementary material for: Learning in Auctions: Regret is Hard, Envy is Easy
Source: arXiv:1511.01411 source file (2016-04-06)
Supplement: Supplementary file 2 [file appendix-contextual.tex]

\begin{proofof}{Theorem \ref{thm:contextual-regret}}
We will apply Theorem \ref{thm:statistic-regret}. Thus we need to bound $q(\theta)$, $f_-(\theta)$ and $f_+(\theta)$.

As we argued in Equation \eqref{eqn:bounded-stat-change}, we have that for any $\theta=(c,r)$: $q(\theta)\leq \|r\|_1\leq N\cdot H$. Thus for any sequence with $r_j^t\in [0,H]$ we get $D=N\cdot H$. Moreover, for any $\theta=(c,r)$, $u(\pi,\theta)\in [-\|r\|_{\infty},\|r\|_{\infty}]$. 

If we denote with $z\in \R^N$ a vector whose coordinate is distributed independently according to a symmetric exponential distribution, then since our random sequence $\{x\}$ is generated by adding $d$ such vectors, one for each context, we get:
\begin{equation}
 \E_{\{x\}}\left[\sum_{x^{\tau}\in \{x\}} \left(f_-(x^\tau)+f_+(x^\tau)\right)\right] = d \cdot 2\cdot \E_{z}\left[ \|z\|_{\infty}\right]
 \end{equation}
$\|z\|_{\infty}$ is the maximum of $N$ independent exponential distributions with parameter $\epsilon$. The expected value of this maximum is upper bounded by $(1+\log(N))/\epsilon$ (see \cite{Kalai2005}). 

Combining all the above we get that the regret is bounded by:
\begin{equation}
\epsilon \cdot H^2 \cdot N \cdot T + d\cdot 2 \cdot \frac{\log(N)+1}{\epsilon}
\end{equation}
By picking $\epsilon = \frac{\sqrt{d\cdot 2 \cdot (\log(N)+1)}}{H\cdot \sqrt{N\cdot T}}$, we get a regret bounded by: $2H\cdot\sqrt{d\cdot 2\cdot (\log(N)+1) \cdot N\cdot T}$ 
\end{proofof}
